# Supplementary material for: Multi-Task Neural Processes
Source: arXiv:2110.14953 source file (2022-03-25)
Supplement: Supplementary file 1 [file appendix_celeba_additional_results_backup.tex]

\begin{figure}[ht!]
    \begin{minipage}{\textwidth}
        \centering
        \scriptsize
        \captionsetup{type=table}
        \caption{Average reconstruction errors (performance) and disagreement of predictions (coherency) on 2D function regression, with varying context size ($m$) and $\gamma = 0$.}
        \vspace{2pt}
        \setlength\tabcolsep{5pt}
        \begin{tabular}{cccc}
            \toprule
            task
            & \multicolumn{3}{c}{{RGB} (performance)} \\
            \cmidrule(lr){1-1} \cmidrule(r){2-4}
            $m$ & 8 & 64 & 256 \\
            \midrule
			STP
			& 0.1461 $\pm$ 0.0014
			& 0.0450 $\pm$ 0.0001
			& 0.0285 $\pm$ 0.0000 \\
			STP+JTP
			& 0.1872 $\pm$ 0.0013
			& 0.0422 $\pm$ 0.0001
			& 0.0255 $\pm$ 0.0001 \\
			MTP
			& \textbf{0.1303} $\pm$ 0.0013
			& \textbf{0.0379} $\pm$ 0.0001
			& \textbf{0.0226} $\pm$ 0.0001 \\
            \bottomrule
        \end{tabular}
        \vspace{4pt}
        
        \begin{tabular}{ccccccc}
            \toprule
            task
            & \multicolumn{3}{c}{{Edge} (performance)}
            & \multicolumn{3}{c}{{Edge} (coherency)} \\
            \cmidrule(lr){1-1} \cmidrule(r){2-4} \cmidrule(r){5-7}
            $m$ & 8 & 64 & 256 & 8 & 64 & 256  \\
            \midrule
			STP
			& 0.0424 $\pm$ 0.0002
			& 0.0244 $\pm$ 0.0001
			& 0.0173 $\pm$ 0.0000
			& 0.0000 $\pm$ 0.0000
			& 0.0000 $\pm$ 0.0000
			& 0.0000 $\pm$ 0.0000\\
			STP+JTP
			& 0.0498 $\pm$ 0.0003
			& 0.0214 $\pm$ 0.0000
			& 0.0148 $\pm$ 0.0000
			& 0.0000 $\pm$ 0.0000
			& 0.0000 $\pm$ 0.0000
			& 0.0000 $\pm$ 0.0000\\
			MTP
			& \textbf{0.0379} $\pm$ 0.0001
			& \textbf{0.0196} $\pm$ 0.0001
			& \textbf{0.0138} $\pm$ 0.0000
			& 0.0000 $\pm$ 0.0000
			& 0.0000 $\pm$ 0.0000
			& 0.0000 $\pm$ 0.0000\\
            \bottomrule
        \end{tabular}
        \vspace{4pt}
        
        \begin{tabular}{ccccccc}
            \toprule
            task
            & \multicolumn{3}{c}{{Segment} (performance)}
            & \multicolumn{3}{c}{{Segment} (coherency)} \\
            \cmidrule(lr){1-1} \cmidrule(r){2-4} \cmidrule(r){5-7}
            $m$ & 8 & 64 & 256 & 8 & 64 & 256  \\
            \midrule
			STP
			& 0.6845 $\pm$ 0.0035
			& 0.4492 $\pm$ 0.0020
			& 0.3741 $\pm$ 0.0012
			& 0.0000 $\pm$ 0.0000
			& 0.0000 $\pm$ 0.0000
			& 0.0000 $\pm$ 0.0000\\
			STP+JTP
			& 0.7608 $\pm$ 0.0018
			& 0.4649 $\pm$ 0.0011
			& 0.4077 $\pm$ 0.0014
			& 0.0000 $\pm$ 0.0000
			& 0.0000 $\pm$ 0.0000
			& 0.0000 $\pm$ 0.0000\\
			MTP
			& \textbf{0.6335} $\pm$ 0.0010
			& \textbf{0.4159} $\pm$ 0.0021
			& \textbf{0.3710} $\pm$ 0.0005
			& 0.0000 $\pm$ 0.0000
			& 0.0000 $\pm$ 0.0000
			& 0.0000 $\pm$ 0.0000\\
            \bottomrule
        \end{tabular}
        \vspace{4pt}
        
        \begin{tabular}{ccccccc}
            \toprule
            task
            & \multicolumn{3}{c}{{PNCC} (performance)}
            & \multicolumn{3}{c}{{PNCC} (coherency)} \\
            \cmidrule(lr){1-1} \cmidrule(r){2-4} \cmidrule(r){5-7}
            $m$ & 8 & 64 & 256 & 8 & 64 & 256  \\
            \midrule
			STP
			& 0.0632 $\pm$ 0.0011
			& 0.0076 $\pm$ 0.0001
			& 0.0043 $\pm$ 0.0000
			& 0.0000 $\pm$ 0.0000
			& 0.0000 $\pm$ 0.0000
			& 0.0000 $\pm$ 0.0000\\
			STP+JTP
			& 0.0929 $\pm$ 0.0012
			& 0.0097 $\pm$ 0.0002
			& 0.0052 $\pm$ 0.0000
			& 0.0000 $\pm$ 0.0000
			& 0.0000 $\pm$ 0.0000
			& 0.0000 $\pm$ 0.0000\\
			MTP
			& \textbf{0.0565} $\pm$ 0.0009
			& \textbf{0.0049} $\pm$ 0.0001
			& \textbf{0.0029} $\pm$ 0.0000
			& 0.0000 $\pm$ 0.0000
			& 0.0000 $\pm$ 0.0000
			& 0.0000 $\pm$ 0.0000\\
            \bottomrule
        \end{tabular}
        \label{tab:tasks_image_gamma_0}
    \end{minipage}
    % \vspace{4pt}
    
    % \begin{minipage}{\textwidth}
    %     \centering
    %     \includegraphics[width=\linewidth]{figures/celeba_qualitative_supplementary_dr0.pdf}
    %     \vspace{-4pt}
    %     \captionsetup{type=figure}
    %     \caption{Qualitative results on 2D function regression. ($\gamma=0$)}
    %     \label{fig:qualitative_2d_dr0}
    % \end{minipage}
\end{figure}


\begin{figure}[ht!]
    \begin{minipage}{\textwidth}
        \centering
        \scriptsize
        \captionsetup{type=table}
        \caption{Average reconstruction errors (performance) and disagreement of predictions (coherency) on 2D function regression, with varying context size ($m$) and $\gamma = 0.25$.}
        \vspace{5pt}
        \setlength\tabcolsep{5pt}
        \begin{tabular}{cccc}
            \toprule
            task
            & \multicolumn{3}{c}{{RGB} (performance)} \\
            \cmidrule(lr){1-1} \cmidrule(r){2-4}
            $m$ & 8 & 64 & 256 \\
            \midrule
			STP
			& 0.1637 $\pm$ 0.0021
			& 0.0524 $\pm$ 0.0002
			& 0.0306 $\pm$ 0.0001 \\
			STP+JTP
			& 0.1948 $\pm$ 0.0012
			& 0.0527 $\pm$ 0.0003
			& 0.0345 $\pm$ 0.0001 \\
			MTP
			& \textbf{0.1452} $\pm$ 0.0015
			& \textbf{0.0442} $\pm$ 0.0002
			& \textbf{0.0242} $\pm$ 0.0000 \\
            \bottomrule
        \end{tabular}
        \vspace{4pt}
        
        \begin{tabular}{ccccccc}
            \toprule
            task
            & \multicolumn{3}{c}{{Edge} (performance)}
            & \multicolumn{3}{c}{{Edge} (coherency)} \\
            \cmidrule(lr){1-1} \cmidrule(r){2-4} \cmidrule(r){5-7}
            $m$ & 8 & 64 & 256 & 8 & 64 & 256  \\
            \midrule
			STP
			& 0.0437 $\pm$ 0.0002
			& 0.0268 $\pm$ 0.0001
			& 0.0183 $\pm$ 0.0000
			& 0.0000 $\pm$ 0.0000
			& 0.0000 $\pm$ 0.0000
			& 0.0000 $\pm$ 0.0000\\
			STP+JTP
			& 0.0502 $\pm$ 0.0002
			& 0.0247 $\pm$ 0.0001
			& 0.0185 $\pm$ 0.0000
			& 0.0000 $\pm$ 0.0000
			& 0.0000 $\pm$ 0.0000
			& 0.0000 $\pm$ 0.0000\\
			MTP
			& \textbf{0.0397} $\pm$ 0.0001
			& \textbf{0.0216} $\pm$ 0.0001
			& \textbf{0.0146} $\pm$ 0.0000
			& 0.0000 $\pm$ 0.0000
			& 0.0000 $\pm$ 0.0000
			& 0.0000 $\pm$ 0.0000\\
            \bottomrule
        \end{tabular}
        \vspace{4pt}
        
        \begin{tabular}{ccccccc}
            \toprule
            task
            & \multicolumn{3}{c}{{Segment} (performance)}
            & \multicolumn{3}{c}{{Segment} (coherency)} \\
            \cmidrule(lr){1-1} \cmidrule(r){2-4} \cmidrule(r){5-7}
            $m$ & 8 & 64 & 256 & 8 & 64 & 256  \\
            \midrule
			STP
			& 0.7168 $\pm$ 0.0044
			& 0.4742 $\pm$ 0.0015
			& 0.3878 $\pm$ 0.0015
			& 0.0000 $\pm$ 0.0000
			& 0.0000 $\pm$ 0.0000
			& 0.0000 $\pm$ 0.0000\\
			STP+JTP
			& 0.8003 $\pm$ 0.0016
			& 0.5013 $\pm$ 0.0014
			& 0.4404 $\pm$ 0.0014
			& 0.0000 $\pm$ 0.0000
			& 0.0000 $\pm$ 0.0000
			& 0.0000 $\pm$ 0.0000\\
			MTP
			& \textbf{0.6648} $\pm$ 0.0017
			& \textbf{0.4325} $\pm$ 0.0013
			& \textbf{0.3774} $\pm$ 0.0005
			& 0.0000 $\pm$ 0.0000
			& 0.0000 $\pm$ 0.0000
			& 0.0000 $\pm$ 0.0000\\
            \bottomrule
        \end{tabular}
        \vspace{4pt}
        
        \begin{tabular}{ccccccc}
            \toprule
            task
            & \multicolumn{3}{c}{{PNCC} (performance)}
            & \multicolumn{3}{c}{{PNCC} (coherency)} \\
            \cmidrule(lr){1-1} \cmidrule(r){2-4} \cmidrule(r){5-7}
            $m$ & 8 & 64 & 256 & 8 & 64 & 256  \\
            \midrule
			STP
			& 0.0772 $\pm$ 0.0012
			& 0.0092 $\pm$ 0.0001
			& 0.0050 $\pm$ 0.0000
			& 0.0000 $\pm$ 0.0000
			& 0.0000 $\pm$ 0.0000
			& 0.0000 $\pm$ 0.0000\\
			STP+JTP
			& 0.1174 $\pm$ 0.0022
			& 0.0140 $\pm$ 0.0002
			& 0.0076 $\pm$ 0.0001
			& 0.0000 $\pm$ 0.0000
			& 0.0000 $\pm$ 0.0000
			& 0.0000 $\pm$ 0.0000\\
			MTP
			& \textbf{0.0646} $\pm$ 0.0011
			& \textbf{0.0061} $\pm$ 0.0001
			& \textbf{0.0031} $\pm$ 0.0000
			& 0.0000 $\pm$ 0.0000
			& 0.0000 $\pm$ 0.0000
			& 0.0000 $\pm$ 0.0000\\
            \bottomrule
        \end{tabular}
        \label{tab:tasks_image_gamma_0.25}
    \end{minipage}
    \vspace{4pt}
    
    % \begin{minipage}{\textwidth}
    %     \centering
    %     \includegraphics[width=\linewidth]{figures/celeba_qualitative_supplementary_dr0.25.pdf}
    %     \captionsetup{type=figure}
    %     \caption{Qualitative results on 2D function regression. ($\gamma=0.25$)}
    %     \label{fig:qualitative_2d_dr0.25}
    % \end{minipage}    
\end{figure}


\begin{figure}[ht!]
    \begin{minipage}{\textwidth}
        \centering
        \scriptsize
        \captionsetup{type=table}
        \caption{Average reconstruction errors (performance) and disagreement of predictions (coherency) on 2D function regression, with varying context size ($m$) and $\gamma = 0.5$.}
        \vspace{5pt}
        \setlength\tabcolsep{5pt}
        \begin{tabular}{cccc}
            \toprule
            task
            & \multicolumn{3}{c}{{RGB} (performance)} \\
            \cmidrule(lr){1-1} \cmidrule(r){2-4}
            $m$ & 8 & 64 & 256 \\
            \midrule
			STP
			& 0.1838 $\pm$ 0.0022
			& 0.0669 $\pm$ 0.0004
			& 0.0355 $\pm$ 0.0001 \\
			JTP
			& 0.2089 $\pm$ 0.0023
			& 0.0636 $\pm$ 0.0004
			& 0.0372 $\pm$ 0.0001 \\
			MTP
			& \textbf{0.1630} $\pm$ 0.0018
			& \textbf{0.0576} $\pm$ 0.0002
			& \textbf{0.0284} $\pm$ 0.0001 \\
            \bottomrule
        \end{tabular}
        \vspace{4pt}
        
        \begin{tabular}{ccccccc}
            \toprule
            task
            & \multicolumn{3}{c}{{Edge} (performance)}
            & \multicolumn{3}{c}{{Edge} (coherency)} \\
            \cmidrule(lr){1-1} \cmidrule(r){2-4} \cmidrule(r){5-7}
            $m$ & 8 & 64 & 256 & 8 & 64 & 256  \\
            \midrule
			STP
			& 0.0447 $\pm$ 0.0002
			& 0.0304 $\pm$ 0.0002
			& 0.0205 $\pm$ 0.0000
			& 0.0000 $\pm$ 0.0000
			& 0.0000 $\pm$ 0.0000
			& 0.0000 $\pm$ 0.0000\\
			JTP
			& 0.0508 $\pm$ 0.0003
			& 0.0272 $\pm$ 0.0001
			& 0.0195 $\pm$ 0.0000
			& 0.0000 $\pm$ 0.0000
			& 0.0000 $\pm$ 0.0000
			& 0.0000 $\pm$ 0.0000\\
			MTP
			& \textbf{0.0416} $\pm$ 0.0002
			& \textbf{0.0249} $\pm$ 0.0001
			& \textbf{0.0160} $\pm$ 0.0000
			& 0.0000 $\pm$ 0.0000
			& 0.0000 $\pm$ 0.0000
			& 0.0000 $\pm$ 0.0000\\
            \bottomrule
        \end{tabular}
        \vspace{4pt}
        
        \begin{tabular}{ccccccc}
            \toprule
            task
            & \multicolumn{3}{c}{{Segment} (performance)}
            & \multicolumn{3}{c}{{Segment} (coherency)} \\
            \cmidrule(lr){1-1} \cmidrule(r){2-4} \cmidrule(r){5-7}
            $m$ & 8 & 64 & 256 & 8 & 64 & 256  \\
            \midrule
			STP
			& 0.7551 $\pm$ 0.0016
			& 0.5139 $\pm$ 0.0008
			& 0.4106 $\pm$ 0.0023
			& 0.0000 $\pm$ 0.0000
			& 0.0000 $\pm$ 0.0000
			& 0.0000 $\pm$ 0.0000\\
			JTP
			& 0.8243 $\pm$ 0.0022
			& 0.5209 $\pm$ 0.0025
			& 0.4471 $\pm$ 0.0016
			& 0.0000 $\pm$ 0.0000
			& 0.0000 $\pm$ 0.0000
			& 0.0000 $\pm$ 0.0000\\
			MTP
			& \textbf{0.7056} $\pm$ 0.0027
			& \textbf{0.4606} $\pm$ 0.0018
			& \textbf{0.3888} $\pm$ 0.0013
			& 0.0000 $\pm$ 0.0000
			& 0.0000 $\pm$ 0.0000
			& 0.0000 $\pm$ 0.0000\\
            \bottomrule
        \end{tabular}
        \vspace{4pt}
        
        \begin{tabular}{ccccccc}
            \toprule
            task
            & \multicolumn{3}{c}{{PNCC} (performance)}
            & \multicolumn{3}{c}{{PNCC} (coherency)} \\
            \cmidrule(lr){1-1} \cmidrule(r){2-4} \cmidrule(r){5-7}
            $m$ & 8 & 64 & 256 & 8 & 64 & 256  \\
            \midrule
			STP
			& 0.0958 $\pm$ 0.0010
			& 0.0136 $\pm$ 0.0002
			& 0.0067 $\pm$ 0.0001
			& 0.0000 $\pm$ 0.0000
			& 0.0000 $\pm$ 0.0000
			& 0.0000 $\pm$ 0.0000\\
			JTP
			& 0.1344 $\pm$ 0.0022
			& 0.0166 $\pm$ 0.0003
			& 0.0085 $\pm$ 0.0001
			& 0.0000 $\pm$ 0.0000
			& 0.0000 $\pm$ 0.0000
			& 0.0000 $\pm$ 0.0000\\
			MTP
			& \textbf{0.0726} $\pm$ 0.0009
			& \textbf{0.0095} $\pm$ 0.0002
			& \textbf{0.0037} $\pm$ 0.0001
			& 0.0000 $\pm$ 0.0000
			& 0.0000 $\pm$ 0.0000
			& 0.0000 $\pm$ 0.0000\\
            \bottomrule
        \end{tabular}
        \label{tab:tasks_image_gamma_0.5}
    \end{minipage}
    \vspace{4pt}
    
    % \begin{minipage}{\textwidth}
    %     \centering
    %     \includegraphics[width=\linewidth]{figures/celeba_qualitative_supplementary_dr0.5.pdf}
    %     \captionsetup{type=figure}
    %     \caption{Qualitative results on 2D function regression. ($\gamma=0.5$)}
    %     \label{fig:qualitative_2d_dr0.5}
    % \end{minipage}    
\end{figure}


\begin{figure}[ht!]
    \begin{minipage}{\textwidth}
        \centering
        \scriptsize
        \captionsetup{type=table}
        \caption{Average reconstruction errors (performance) and disagreement of predictions (coherency) on 2D function regression, with varying context size ($m$) and $\gamma = 0.75$.}
        \vspace{5pt}
        \setlength\tabcolsep{5pt}
        \begin{tabular}{cccc}
            \toprule
            task
            & \multicolumn{3}{c}{{RGB} (performance)} \\
            \cmidrule(lr){1-1} \cmidrule(r){2-4}
            $m$ & 8 & 64 & 256 \\
            \midrule
			STP
			& 0.2090 $\pm$ 0.0021
			& 0.1006 $\pm$ 0.0005
			& 0.0503 $\pm$ 0.0002 \\
			STP+JTP
			& 0.2273 $\pm$ 0.0031
			& 0.0928 $\pm$ 0.0003
			& 0.0466 $\pm$ 0.0001 \\
			MTP
			& \textbf{0.1856} $\pm$ 0.0017
			& \textbf{0.0915} $\pm$ 0.0004
			& \textbf{0.0442} $\pm$ 0.0003 \\
            \bottomrule
        \end{tabular}
        \vspace{4pt}
        
        \begin{tabular}{ccccccc}
            \toprule
            task
            & \multicolumn{3}{c}{{Edge} (performance)}
            & \multicolumn{3}{c}{{Edge} (coherency)} \\
            \cmidrule(lr){1-1} \cmidrule(r){2-4} \cmidrule(r){5-7}
            $m$ & 8 & 64 & 256 & 8 & 64 & 256  \\
            \midrule
			STP
			& 0.0453 $\pm$ 0.0002
			& 0.0360 $\pm$ 0.0001
			& 0.0254 $\pm$ 0.0001
			& 0.0000 $\pm$ 0.0000
			& 0.0000 $\pm$ 0.0000
			& 0.0000 $\pm$ 0.0000\\
			STP+JTP
			& 0.0515 $\pm$ 0.0001
			& 0.0324 $\pm$ 0.0000
			& 0.0223 $\pm$ 0.0001
			& 0.0000 $\pm$ 0.0000
			& 0.0000 $\pm$ 0.0000
			& 0.0000 $\pm$ 0.0000\\
			MTP
			& \textbf{0.0436} $\pm$ 0.0002
			& \textbf{0.0311} $\pm$ 0.0001
			& \textbf{0.0197} $\pm$ 0.0000
			& 0.0000 $\pm$ 0.0000
			& 0.0000 $\pm$ 0.0000
			& 0.0000 $\pm$ 0.0000\\
            \bottomrule
        \end{tabular}
        \vspace{4pt}
        
        \begin{tabular}{ccccccc}
            \toprule
            task
            & \multicolumn{3}{c}{{Segment} (performance)}
            & \multicolumn{3}{c}{{Segment} (coherency)} \\
            \cmidrule(lr){1-1} \cmidrule(r){2-4} \cmidrule(r){5-7}
            $m$ & 8 & 64 & 256 & 8 & 64 & 256  \\
            \midrule
			STP
			& 0.7975 $\pm$ 0.0028
			& 0.5921 $\pm$ 0.0025
			& 0.4637 $\pm$ 0.0019
			& 0.0000 $\pm$ 0.0000
			& 0.0000 $\pm$ 0.0000
			& 0.0000 $\pm$ 0.0000\\
			STP+JTP
			& 0.8512 $\pm$ 0.0008
			& 0.5708 $\pm$ 0.0012
			& 0.4680 $\pm$ 0.0011
			& 0.0000 $\pm$ 0.0000
			& 0.0000 $\pm$ 0.0000
			& 0.0000 $\pm$ 0.0000\\
			MTP
			& \textbf{0.7584} $\pm$ 0.0017
			& \textbf{0.5259} $\pm$ 0.0012
			& \textbf{0.4158} $\pm$ 0.0010
			& 0.0000 $\pm$ 0.0000
			& 0.0000 $\pm$ 0.0000
			& 0.0000 $\pm$ 0.0000\\
            \bottomrule
        \end{tabular}
        \vspace{4pt}
        
        \begin{tabular}{ccccccc}
            \toprule
            task
            & \multicolumn{3}{c}{{PNCC} (performance)}
            & \multicolumn{3}{c}{{PNCC} (coherency)} \\
            \cmidrule(lr){1-1} \cmidrule(r){2-4} \cmidrule(r){5-7}
            $m$ & 8 & 64 & 256 & 8 & 64 & 256  \\
            \midrule
			STP
			& 0.1191 $\pm$ 0.0013
			& 0.0255 $\pm$ 0.0005
			& 0.0108 $\pm$ 0.0001
			& 0.0000 $\pm$ 0.0000
			& 0.0000 $\pm$ 0.0000
			& 0.0000 $\pm$ 0.0000\\
			STP+JTP
			& 0.1544 $\pm$ 0.0021
			& 0.0264 $\pm$ 0.0005
			& 0.0113 $\pm$ 0.0001
			& 0.0000 $\pm$ 0.0000
			& 0.0000 $\pm$ 0.0000
			& 0.0000 $\pm$ 0.0000\\
			MTP
			& \textbf{0.0754} $\pm$ 0.0008
			& \textbf{0.0212} $\pm$ 0.0003
			& \textbf{0.0096} $\pm$ 0.0001
			& 0.0000 $\pm$ 0.0000
			& 0.0000 $\pm$ 0.0000
			& 0.0000 $\pm$ 0.0000\\
            \bottomrule
        \end{tabular}
        \label{tab:tasks_image_gamma_0.75}
    \end{minipage}
    \vspace{4pt}
    
    % \begin{minipage}{\textwidth}
    %     \centering
    %     \includegraphics[width=\linewidth]{figures/celeba_qualitative_supplementary_dr0.75.pdf}
    %     \captionsetup{type=figure}
    %     \caption{Qualitative results on 2D function regression. ($\gamma=0.75$)}
    %     \label{fig:qualitative_2d_dr0.75}
    % \end{minipage}    
\end{figure}

% \begin{table}[ht!]
%     \small
%     \centering
%     \caption{Relative performance gain with 5 different random seeds (\%).}
%     \setlength\tabcolsep{4pt}
%     \begin{tabular}{ccccc}
%         \toprule
%         Source $\backslash$ Target & {RGB} & {Edge} & {Segment} & {PNCC} \\
%         \midrule
%         {RGB} &
%         - & \textbf{53.02 $\pm$ 4.71} & 8.73 $\pm$ 6.50 & 18.57 $\pm$ 12.94 \\
%         {Edge} &
%         \textbf{6.35 $\pm$ 1.95} & - & 8.18 $\pm$ 6.63 & 15.70 $\pm$ 13.11 \\
%         {Segment} &
%         5.13 $\pm$ 2.04 & 33.30 $\pm$ 23.94 & - & \textbf{29.24 $\pm$ 2.62} \\
%         {PNCC} &
%         5.58 $\pm$ 2.53 & 31.88 $\pm$ 23.64 & \textbf{15.88 $\pm$ 2.21} & - \\
%         \bottomrule
%     \end{tabular}
%     \label{tab:task_transfer_image_5seeds}
% \end{table}
